# Supplementary material for: GenMix: Combining Generative and Mixture Data Augmentation for Medical Image Classification
Source: arXiv:2405.20650 source file (2024-07-16)
Supplement: Supplementary file 1 [file x_supplement.tex]

\section{Additional Tables and Figures}
